# Supplementary material for: Decoupling carrier concentration and electron-phonon coupling in oxide heterostructures observed with resonant inelastic x-ray scattering
Source: arXiv:1810.08327 ancillary file (2018-10-19)
Supplement: Supplementary file 1 [file Supplemenal.pdf]

# Supplemental Materials: Decoupling carrier concentration from electron-phonon coupling in oxide heterostructures

D. Meyers,<sup>1,\*</sup> Ken Nakatsukasa,<sup>2</sup> Sai Mu,<sup>3</sup> Lin Hao,<sup>2</sup> Junyi Yang,<sup>2</sup> Yue Cao,<sup>1</sup> G. Fabbri,<sup>4</sup> Hu Miao,<sup>1</sup> J. Pelliciani,<sup>5</sup> D. McNally,<sup>5</sup> M. Dantz,<sup>5</sup> E. Paris,<sup>5</sup> E. Karapetrova,<sup>4</sup> Yongseong Choi,<sup>4</sup> D. Haskel,<sup>4</sup> P. Shafer,<sup>6</sup> E. Arenholz,<sup>6</sup> Thorsten Schmitt,<sup>5</sup> Tom Berlijn,<sup>7,8,†</sup> S. Johnston,<sup>2,9,‡</sup> Jian Liu,<sup>2,§</sup> and M. P. M. Dean<sup>1,¶</sup>

<sup>1</sup>*Department of Condensed Matter Physics and Materials Science,  
Brookhaven National Laboratory, Upton, New York 11973, USA*

<sup>2</sup>*Department of Physics and Astronomy, University of Tennessee, Knoxville, Tennessee 37996, USA*

<sup>3</sup>*Department of Condensed Matter Physics and Materials Science,  
Oak Ridge National Laboratory, Oak Ridge, Tennessee 37830, USA*

<sup>4</sup>*Advanced Photon Source, Argonne National Laboratory, Argonne, Illinois 60439, USA*

<sup>5</sup>*Research Department Synchrotron Radiation and Nanotechnology,  
Paul Scherrer Institut, CH-5232 Villigen PSI, Switzerland*

<sup>6</sup>*Advanced Light Source, Lawrence Berkeley National Laboratory, Berkeley, CA 94720, USA*

<sup>7</sup>*Center for Nanophase Materials Sciences, Oak Ridge National Laboratory, Oak Ridge, TN 37831, USA*

<sup>8</sup>*Computational Science and Engineering Division,  
Oak Ridge National Laboratory, Oak Ridge, Tennessee 37831, USA*

<sup>9</sup>*Joint Institute of Advanced Materials at The University of Tennessee, Knoxville, Tennessee 37996, USA*

(Dated: October 19, 2018)

## CONTENTS

|                                                      |   |
|------------------------------------------------------|---|
| I. Additional characterization                       | 2 |
| A. Transport                                         | 2 |
| B. X-ray absorption spectroscopy                     | 2 |
| II. RIXS data                                        | 2 |
| III. Fitting routine                                 | 3 |
| A. Constant background                               | 3 |
| B. No background                                     | 3 |
| IV. Octahedral tilting                               | 4 |
| A. Experiment                                        | 4 |
| B. Supporting Theory Calculations                    | 4 |
| V. Additional density functional theory calculations | 5 |
| References                                           | 7 |

This supplemental materials contains additional transport and X-ray absorption spectroscopy (XAS) data for the samples, additional comparison of the elastic and phonon features, details of the fitting routine used along with an alternative background fitting which yields qualitatively consistent results, experimental and theoretical analysis of the octahedral tilting and it's effect on the electron-phonon coupling (EPC), and further details of the density functional theory (DFT) calculations shown in the manuscript.

---

\* [dmeyers@bnl.gov](mailto:dmeyers@bnl.gov)

† [tberlijn@gmail.com](mailto:tberlijn@gmail.com)

‡ [sjohn145@utk.edu](mailto:sjohn145@utk.edu)

§ [jianliu@utk.edu](mailto:jianliu@utk.edu)

¶ [mdean@bnl.gov](mailto:mdean@bnl.gov)

## I. ADDITIONAL CHARACTERIZATION

### A. Transport

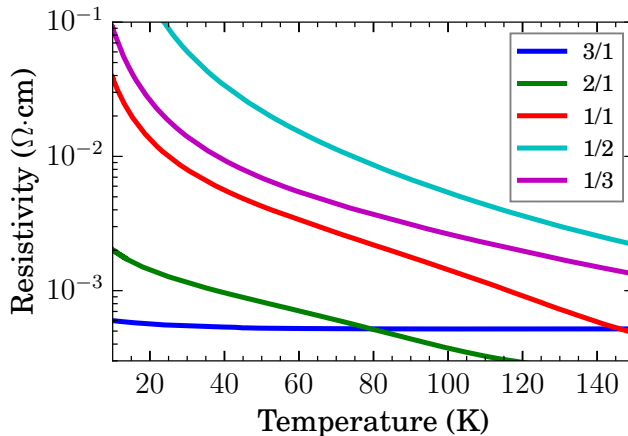

FIG. 1. Resistivity data for all samples at low T.

Resistivity data for all samples is shown in Fig. 1. All samples show insulating behavior except 3SrIrO<sub>3</sub>/1SrTiO<sub>3</sub>, which shows semi-conducting behavior similar to pure SrIrO<sub>3</sub> films. Previous studies of doped STO crystals show that doping by even 0.01% reduces the residual resistivity to  $\sim 10^{-4} \Omega \cdot \text{cm}$ . We therefore estimate that the STO layers likely have minimal ( $< 0.01\%$ ) or no charge doping. [1]. Furthermore, the drop in EPC is observed for the still clearly insulating  $n = m = 1$  SL, while the majority SrIrO<sub>3</sub> (SIO) SLs show very similar EPC despite their less insulating nature. This indicates the change in resistivity is mostly driven by the relative confinement of the Ir  $d$ -states. This is consistent with theoretical findings, which show a lowering of the electronic band gap in the Ir  $d$ -states with increasing Ir layer thickness, while the Ti  $d$ -states remain unoccupied [2].

### B. X-ray absorbtion spectroscopy

XAS is a sensitive technique for detecting changes in valence. To further test for charge transfer, we measured the full x-ray absorption spectra at the Ti L-edge, O K-edge, and Ir L<sub>3</sub>-edge for all of the samples in the series, as shown in Fig. 2. The Ti and O data were taken in total electron yield, while the Ir data was taken in total florescence yield. Minimal deviations in line shape or peak positions occur in the spectra, which would signal valence changes as one moves to the SrTiO<sub>3</sub> (STO) minority samples, as seen in Ti<sup>3+</sup> samples [3–7]. A reference Ti 3<sup>+</sup> spectra is provided in Fig. 2(a). The x-ray attenuation length here, accounting for resonance and incidence angle (30°), is 40 – 60 nm, on the order of our film thickness. The electron escape depth is only about 4 nm indicating the vast majority of our Ti L-edge signal comes from the STO layers within the superlattice (SL) and contains little to no STO substrate signal. The O K-edge attenuation length is 50 – 70 nm, slightly thicker than our samples. The Ir L<sub>3</sub> data shows no multi-valence broadening for the 1SIO/3STO sample as would be expected if carriers were being pulled from the SIO layers. The energy was calibrated with a Pt reference. XAS data for the Ti L-edge and O K-edge was taken at beamline 4.0.2 of the Advanced Light Source of Lawrence Berkeley National Laboratory [8]. XAS data for the Ir L-edge was taken at beamline 4-ID-D of the Advanced Photon Source at Argonne National Laboratory.

## II. RIXS DATA

Measurements were taken at 135° scattering angle. All spectra were corrected for self-absorption effects. To confirm the change in relative intensities of the phonon features is not due to a change in elastic features, comparison of the resonant inelastic x-ray scattering (RIXS) spectra after subtraction of the elastic feature is presented in Fig. 3, showing the same trend as in Fig. 2(b) of the manuscript.

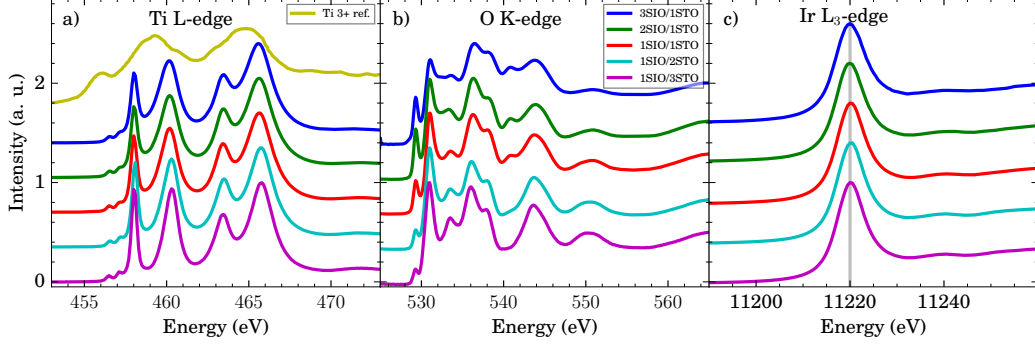

FIG. 2. a) Ti L-edge, b) O K-edge, and c) Ir  $L_3$ -edge XAS spectra, all showing no discernible charge transfer from the Ir to the Ti  $d$ -states.

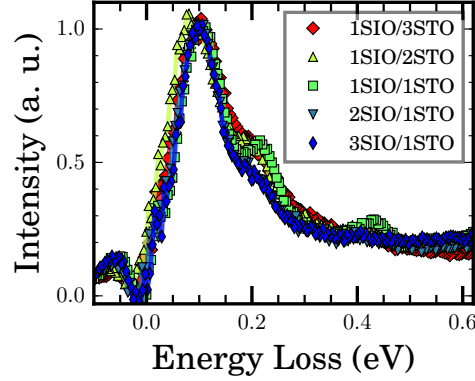

FIG. 3. RIXS data for each sample with the fit elastic contribution removed.

### III. FITTING ROUTINE

#### A. Constant background

All spectra were fit with three features, (i) a Gaussian for the elastic line, (ii) the Ament phonon function, and (iii) a weak background constant above 0 energy loss. The fitting was performed between -50 and 400 meV. For (i), all parameters were allowed to freely float. For (ii),  $\omega_{det}$  was defined to be 0 as each sample was carefully calibrated to the maximum of the resonance,  $\Gamma$  was set to the O K-edge core-hole lifetime (220 meV) [9], the resolution was set by the instrumental resolution measured with carbon tape, and the remaining parameters were allowed to float. The full set of free parameters is then:  $g$  (dimensionless electron-phonon coupling strength),  $I_0$  (multiplicative intensity normalization),  $\omega_0$  (phonon frequency), the intrinsic phonon width, and an x-axis offset due to drifts of the zero energy loss position. For (iii), the intensity of the background was set by the residual intensity above 1.5 eV energy loss, well beyond any discernible features, similar to what was done previously [10, 11].

#### B. No background

Alternatively, a fit to the first four phonon excitations with appreciable spectral weight can be done with no constant background. In this case, the predicted phonon excitations above the 4th or fifth satellite feature no longer match the measured spectra, and this region is taken as unfit low-energy excitations, as done by Lee *et al.* [12]. This full analysis is shown in Fig. 4. As can be seen, the end result shows the same general trend in  $M$  as function of layering, though the overall magnitude is larger and the substrate no longer matches the majority STO layer samples, making this seem a less reliable method to fit the data. Using this method, however, the changes in  $\omega_0$  are smaller.

## IV. OCTAHEDRAL TILTING

### A. Experiment

We investigated the rotations of the octahedra within the entire set of SLs using synchrotron-based X-ray diffraction (XRD), as shown in Fig. 4(a). XRD data was measured at the 33-BM beamline of the Advanced Photon Source at Argonne National Laboratory. These half order peaks correspond to rotations about the  $a$ - $b$  axes, which are absent in bulk STO. Broad features originate from the films whereas the stronger, sharper peaks are from the STO substrates. Samples with  $n < m$  show only very small features as lower  $L$ -value shoulders to the substrate peak. However, with  $n = m$  a film feature becomes more distinguishable, becoming an order of magnitude stronger for  $n > m$ . As the degree of rotation is proportional to the XRD amplitude, these results show only very small rotations about the  $a$ - $b$  axes exists for  $n < m$ , with small rotations appearing for  $n = m$ , and largest rotations for  $n = 2, 3$  that appear to be nearly identical, Fig. 5. However, our measurements do not unambiguously identify whether the system is  $a^-a^-c^-$  or  $a^-a^-c^+$  in the Glazer notation [13]. XRD measured lattice constants give an approximate value of  $8^\circ$  for all  $c$ -axis rotations as was done previously [2, 14]. Based on the scattered intensities of the (0.5 0.5 1.5) reflection Fig. 5, we also conclude the  $n > m$  samples host  $a$ - $b$ -axis rotations between  $5$ - $15^\circ$ , the  $n = m$  sample around  $1$ - $2^\circ$ , and the  $n < m$  samples less than  $1^\circ$ .

### B. Supporting Theory Calculations

To theoretically investigate the effects of the octahedral tilts we compute their influence on the EPC in bulk STO to model the situation in the SLs. This should be a reasonable approximation, given that Fig. 4 in the manuscript shows the  $\text{LO}_4$  phonon excitations observed in RIXS reside in the STO layers.

For these calculations we used density functional perturbation theory (DFPT), implemented in Quantum Espresso [15] with the Perdew-Burke-Ernzerhof exchange-correlation (PBE) functional and the GBRV ultrasoft pseudopotentials [16]. In each calculation, we used a  $12 \times 12 \times 8$   $\mathbf{k}$ -point grid, and an energy cutoff of 40 and 400 Ry were chosen for the wavefunction and electron density, respectively. The following standard formula for the EPC was used:

$$\lambda_{\mathbf{q}} = \frac{2}{N(\epsilon_s)\omega_{\mathbf{q}}} \sum_{ij} \int \frac{d^3k}{V_{BZ}} |g_{i,j}(\mathbf{q}, \mathbf{k})|^2 \delta(\epsilon_{\mathbf{q},i} - \epsilon_s) \delta(\epsilon_{\mathbf{q}+\mathbf{k},j} - \epsilon_s), \quad (1)$$

where  $\omega_{\mathbf{q}}$  and  $\epsilon_{\mathbf{k}}$  are the phonon and electron dispersions,  $\mathbf{q}$  and  $\mathbf{k}$  are the wavevectors for phonons and electrons respectively,  $V_{BZ}$  is the volume of the Brillouin zone,  $i, j$  are the band indices,  $N(\omega)$  is the electron density of states,  $g$  is the electron-phonon coupling, and  $\mathbf{q} = (0.24, 0.24, 0)$  (r.l.u.). In the RIXS K-edge process an O-1s core electron is excited into the conduction band. Here we evaluate the EPC at electron energy  $\epsilon_s$  relative to the bottom of the

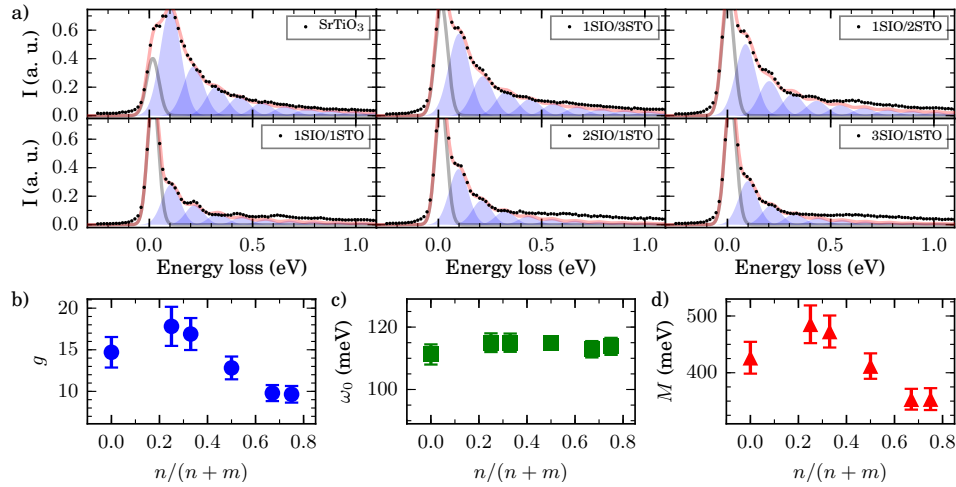

FIG. 4. a) Energy loss spectra at the O K-edge main feature for all samples, including the STO substrate, with fit to the data. The elastic line is shown in grey, the Ament function is shown in blue, and total fit is shown in red. b) The extracted dimensionless EPC strength  $g$  obtained from the fits. c) The extracted  $\omega_0$ , and d) calculated EPC coupling strength  $M$ .

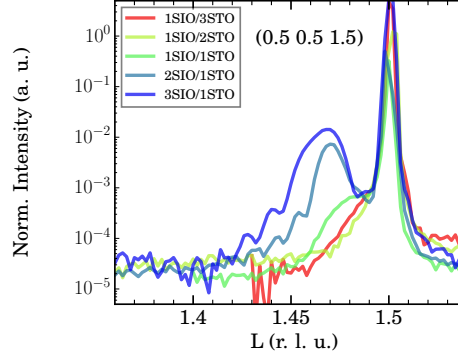

FIG. 5. (0.5 0.5 1.5) and (0.5 0.5 3.5) reflections corresponding to octahedral tilts showing strong structural difference of 2/1 and 3/1 SLs.

conduction band such that the integrated DOS from the bottom of the conduction band to  $\epsilon_s$  is fixed between the different calculations. To incorporate the tilting of the  $\text{TiO}_6$  octahedra we used a  $\sqrt{2}a \times \sqrt{2}a \times 2a$  supercell, where we fix the lattice constant  $a = 3.905 \text{ \AA}$  to that of bulk STO. This choice is motivated by the fact that the in-plane lattice constant is fixed to that of the STO substrate in the SLs. Because our XRD measurements could not unambiguously identify whether the tilts were  $a^-a^-c^-$  or  $a^-a^-c^+$  we considered both scenarios. For each case, we tried three tilting angles for  $a^-$  given by  $\alpha = 0^\circ, 4^\circ, 8^\circ$ , and fixed the angle for  $c^-$  and  $c^+$  to  $8^\circ$ . The six resulting structures used in our DFPT calculations are provided in a separate file called “tiltedstructures.txt”. We note that the tilts necessarily induce small distortions of the  $\text{TiO}_6$  octahedra because the lattice constants were fixed. In total there are 60 phonon modes, of which modes 57-60 correspond to the  $\text{LO}_4$  modes observed with RIXS. Their EPCs are shown in Tab. I and II. The calculations show that, within this simplified model, increasing the tilting angle slightly increases the EPC, at a magnitude much smaller than experimentally observed. This shows that the experimentally observed change in tilting angles are not directly responsible for the change in EPC observed with RIXS.

| Mode             | $\alpha = 0^\circ, \epsilon_s = 0.663 \text{ eV}$ |                                    | $\alpha = 4^\circ, \epsilon_s = 0.632 \text{ eV}$ |                                    | $\alpha = 8^\circ, \epsilon_s = 0.548 \text{ eV}$ |                                    |
|------------------|---------------------------------------------------|------------------------------------|---------------------------------------------------|------------------------------------|---------------------------------------------------|------------------------------------|
|                  | $\lambda_{\mathbf{q}}$                            | $\omega_{\mathbf{q}} [\text{meV}]$ | $\lambda_{\mathbf{q}}$                            | $\omega_{\mathbf{q}} [\text{meV}]$ | $\lambda_{\mathbf{q}}$                            | $\omega_{\mathbf{q}} [\text{meV}]$ |
| 57 <sup>th</sup> | 0.273                                             | 88.9                               | 0.281                                             | 87.6                               | 0.304                                             | 84.3                               |
| 58 <sup>th</sup> | 0.039                                             | 90.1                               | 0.041                                             | 88.8                               | 0.051                                             | 85.2                               |
| 59 <sup>th</sup> | 0.022                                             | 96.0                               | 0.024                                             | 93.9                               | 0.031                                             | 88.1                               |
| 60 <sup>th</sup> | 0.001                                             | 97.5                               | 0.001                                             | 95.5                               | 0.003                                             | 90.0                               |

TABLE I. Computed phonon frequency  $\omega_{\mathbf{q}}$  and electron-phonon coupling  $\lambda_{\mathbf{q}}$  evaluated at electron energy  $\epsilon_s$ , phonon momentum  $\mathbf{q} = (0.24, 0.24, 0)$  as a function of tilting angle  $\alpha$  for tilting  $a^-a^-c^-$ .

| Mode             | $\alpha = 0^\circ, \epsilon_s = 0.578 \text{ eV}$ |                                    | $\alpha = 4^\circ, \epsilon_s = 0.565 \text{ eV}$ |                                    | $\alpha = 8^\circ, \epsilon_s = 0.503 \text{ eV}$ |                                    |
|------------------|---------------------------------------------------|------------------------------------|---------------------------------------------------|------------------------------------|---------------------------------------------------|------------------------------------|
|                  | $\lambda_{\mathbf{q}}$                            | $\omega_{\mathbf{q}} [\text{meV}]$ | $\lambda_{\mathbf{q}}$                            | $\omega_{\mathbf{q}} [\text{meV}]$ | $\lambda_{\mathbf{q}}$                            | $\omega_{\mathbf{q}} [\text{meV}]$ |
| 57 <sup>th</sup> | 0.267                                             | 90.0                               | 0.277                                             | 87.6                               | 0.303                                             | 84.1                               |
| 58 <sup>th</sup> | 0.035                                             | 90.1                               | 0.038                                             | 88.8                               | 0.047                                             | 85.2                               |
| 59 <sup>th</sup> | 0.022                                             | 96.1                               | 0.024                                             | 93.9                               | 0.030                                             | 87.9                               |
| 60 <sup>th</sup> | 0.000                                             | 97.6                               | 0.001                                             | 95.5                               | 0.002                                             | 89.9                               |

TABLE II. Computed phonon frequency  $\omega_{\mathbf{q}}$  and electron-phonon coupling  $\lambda_{\mathbf{q}}$  evaluated at electron energy  $\epsilon_s$ , phonon momentum  $\mathbf{q} = (0.24, 0.24, 0)$  as a function of tilting angle  $\alpha$  for tilting  $a^-a^-c^+$ .

## V. ADDITIONAL DENSITY FUNCTIONAL THEORY CALCULATIONS

Here, we provide computational details for the phonon density of states illustrated in Fig. 4 of the manuscript, the calculations of the high-frequency dielectric constant  $\epsilon_\infty$ , and the Born effective charges (BEC). Density functional theory (DFT) calculations were carried out using the projected augmented wave method (PAW) [17] implemented in the Vienna *ab-initio* Simulation Package (VASP) [18, 19]. The employed PAW pseudopotentials correspond to

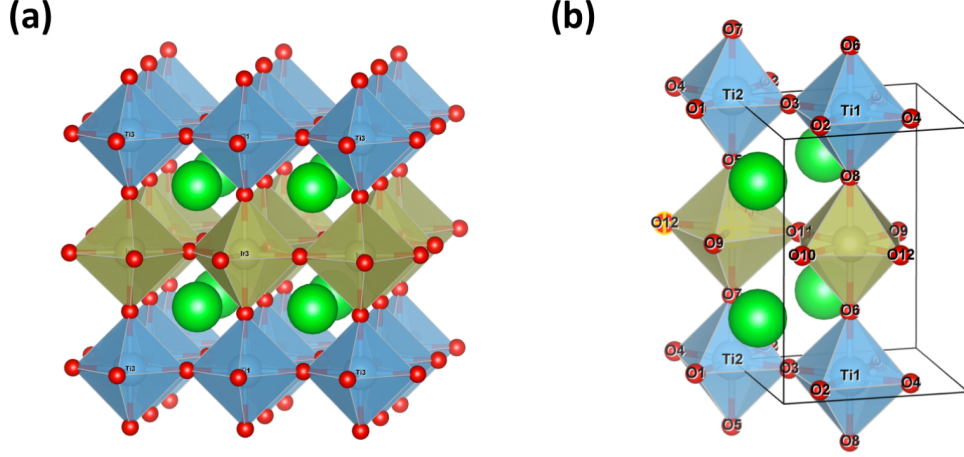

FIG. 6. (a)  $2 \times 2 \times 1$  supercell and (b)  $\sqrt{2} \times \sqrt{2} \times 1$  supercell of  $1\text{SrTiO}_3/1\text{SrIrO}_3$  superlattice. The red spheres are O atoms, the blue spheres are Sr atoms, and Ir atoms and Ti atoms are in the center of the blue and brown octahedral, respectively.

| $\epsilon_\infty$      | $\text{SrTiO}_3$ |     |      | $1\text{SrTiO}_3/1\text{SrIrO}_3$ |      |       |     |          |       |
|------------------------|------------------|-----|------|-----------------------------------|------|-------|-----|----------|-------|
| $\epsilon_\infty^{xx}$ | 5.7              |     |      | 12.5                              |      |       |     |          |       |
| $\epsilon_\infty^{yy}$ | 5.7              |     |      | 12.5                              |      |       |     |          |       |
| $\epsilon_\infty^{zz}$ | 5.7              |     |      | 8.3                               |      |       |     |          |       |
| BEC                    | Sr               | Ti  | O    | Sr                                | Ti   | O(Ti) | Ir  | O(Share) | O(Ir) |
| $Z_{xx}^*$             | 2.49             | 7.7 | -2.1 | 2.49                              | 7.42 | -2    | 4.3 | -1.6     | -1.1  |
| $Z_{yy}^*$             | 2.49             | 7.7 | -6.0 | 2.49                              | 7.42 | -6    | 4.3 | -1.6     | -4.5  |
| $Z_{zz}^*$             | 2.49             | 7.7 | -2.1 | 2.69                              | 8.59 | -2.1  | 4.5 | -5.7     | -1.4  |
| $Z_{xy}^*$             | 0                | 0   | 0    | 0                                 | 1    | 0     | 0   | 0        | 0     |
| $Z_{yx}^*$             | 0                | 0   | 0    | 0                                 | -1   | 0     | 0   | 0        | 0     |

TABLE III. The high-frequency dielectric constant  $\epsilon_\infty$  and the BEC ( $Z^*$ , given in unit of  $e$ ) for  $\text{SrTiO}_3$  and  $1\text{SrTiO}_3/1\text{SrIrO}_3$  superlattice. Three types of O atoms within  $1\text{SrTiO}_3/1\text{SrIrO}_3$  superlattice are selected to show the BEC: O(Ti)/O(Ir) indicates O atom in the Ti/Ir plane, respectively; O(share) denotes O atom shared by Ti and Ir octahedral.

the valence-electron configuration:  $4s^2 4p^6 5s^2$  for Sr,  $3d^3 4s^1$  for Ti,  $6s^1 5d^8$  for Ir, and  $2s^2 2p^4$  for O. Exchange and correlation effects were treated within the generalized gradient approximation (GGA) parametrized by Perdew, Burke and Ernzerhof [20]. A plane wave cutoff energy was set to 520 eV, and a Monkhorst-Pack k-point mesh [21] was used for Brillouin Zone (BZ) integration. The Coulomb correlations of  $5d$  electrons of Ir ions were described by the spherically averaged DFT+ $U$  method [22], and the effective  $U_{\text{eff}} = 2.0$  eV was adopted, consistent with Ref. [23]. In addition, spin polarized calculations were performed in the fully relativistic scheme to include spin-orbit coupling. The resulting ground state corresponds to the antiferromagnetic state with *in-plane* spin moment on Ir  $0.12\mu_B$  and orbital moment on Ir as large as  $0.29\mu_B$ . The internal forces were relaxed to less than  $1 \text{ meV}/\text{\AA}$  without enforcing any symmetry.

To evaluate the partial phonon density of states (pDOS) of the  $1\text{SrTiO}_3/1\text{SrIrO}_3$  superlattice shown in Fig. 5 of the manuscript, we constructed a 40-atom  $2 \times 2 \times 1$  supercell (see Fig. 6a) based on the optimized structure from Ref. [23]. The force constants and the pDOS were calculated using the standard supercell technique with the help of the PHONOPY software [24]. A  $5 \times 5 \times 5$  Monkhorst-Pack  $\mathbf{k}$ -point mesh [21] was used for BZ integration in this particular cell. A  $1 \mu\text{eV}$  energy criterion was employed to converge the total energy in the phonon calculation.

The values of the BEC and  $\epsilon_\infty$  for  $\text{SrTiO}_3$  and  $1\text{SrTiO}_3/1\text{SrIrO}_3$  were calculated using DFPT in VASP. The results are listed in Tab. III. The calculated value of  $\epsilon_\infty$  and the BEC in  $\text{SrTiO}_3$  are consistent with other theories (see Ref. [25] and reference therein). For  $1\text{SrTiO}_3/1\text{SrIrO}_3$ , we used a  $\sqrt{2} \times \sqrt{2} \times 1$  superlattice (see Fig. 6b) to incorporate the AFM order on the Ir sublattice. A BZ integration was performed on a  $4 \times 4 \times 3$  K-point mesh. The results in Tab. III show that the BECs for Sr, Ti, and O(Ti) in  $1\text{SrTiO}_3/1\text{SrIrO}_3$  are close to their values in bulk STO. We note here that the BEC of O(Ti) was rotated by 45 degrees in the  $xy$  plane to better illustrate this resemblance. The average diagonal element of the BEC of Ti/O(Ti) is 1.8/1.4 times larger than that of Ir/O(Ir). The average diagonal

element of  $\epsilon_\infty$  is a factor 1.9 times larger in  $1\text{SrTiO}_3/1\text{SrIrO}_3$  compared to bulk STO.

- 
- [1] X. Lin, B. Fauqué, and K. Behnia, *Science* **349**, 945 (2015).
  - [2] J. Matsuno, K. Ihara, S. Yamamura, H. Wadati, K. Ishii, V. V. Shankar, H.-Y. Kee, and H. Takagi, *Phys. Rev. Lett.* **114**, 247209 (2015).
  - [3] Y. Cao, X. Liu, M. Kareev, D. Choudhury, S. Middey, D. Meyers, J.-W. Kim, P. Ryan, J. Freeland, and J. Chakhalian, *Nature communications* **7** (2016).
  - [4] Y. Cao, S. Y. Park, X. Liu, D. Choudhury, S. Middey, D. Meyers, M. Kareev, P. Shafer, E. Arenholz, and J. Chakhalian, *Applied Physics Letters* **109**, 152905 (2016).
  - [5] Y. Cao, X. Liu, P. Shafer, S. Middey, D. Meyers, M. Kareev, Z. Zhong, J.-W. Kim, P. J. Ryan, E. Arenholz, *et al.*, *npj Quantum Materials* **1**, 16009 (2016).
  - [6] Y. Cao, Z. Yang, M. Kareev, X. Liu, D. Meyers, S. Middey, D. Choudhury, P. Shafer, J. Guo, J. Freeland, *et al.*, *Physical review letters* **116**, 076802 (2016).
  - [7] Y. Cao, P. Shafer, X. Liu, D. Meyers, M. Kareev, S. Middey, J. Freeland, E. Arenholz, and J. Chakhalian, *Applied Physics Letters* **107**, 112401 (2015).
  - [8] See Supplemental Materials at [URL] for experimental and computational details.
  - [9] B. Ravel and M. Newville, *Journal of Synchrotron Radiation* **12**, 537 (2005).
  - [10] S. Moser, S. Fatale, P. Krüger, H. Berger, P. Bugnon, A. Magrez, H. Niwa, J. Miyawaki, Y. Harada, and M. Grioni, *Physical review letters* **115**, 096404 (2015).
  - [11] S. Fatale, S. Moser, J. Miyawaki, Y. Harada, and M. Grioni, *Physical Review B* **94**, 195131 (2016).
  - [12] W. Lee, S. Johnston, B. Moritz, J. Lee, M. Yi, K. Zhou, T. Schmitt, L. Patthey, V. Strocov, K. Kudo, *et al.*, *Physical review letters* **110**, 265502 (2013).
  - [13] A. M. Glazer, *Acta Cryst. A* **31**, 756 (1975).
  - [14] D. Meyers, Y. Cao, G. Fabbri, N. J. Robinson, L. Hao, C. Frederick, N. Traynor, J. Yang, J. Lin, M. Upton, *et al.*, arXiv preprint arXiv:1707.08910 (2017).
  - [15] P. Giannozzi, S. Baroni, N. Bonini, M. Calandra, R. Car, C. Cavazzoni, D. Ceresoli, G. L. Chiarotti, M. Cococcioni, I. Dabo, *et al.*, *Journal of physics: Condensed matter* **21**, 395502 (2009).
  - [16] K. F. Garrity, J. W. Bennett, K. M. Rabe, and D. Vanderbilt, *Computational Materials Science* **81**, 446 (2014).
  - [17] P. E. Blöchl, *Physical review B* **50**, 17953 (1994).
  - [18] G. Kresse and J. Hafner, *Physical Review B* **48**, 13115 (1993).
  - [19] G. Kresse, *Phys. Rev. B* **54**, 11169 (1996).
  - [20] J. P. Perdew, K. Burke, and M. Ernzerhof, *Physical review letters* **77**, 3865 (1996).
  - [21] H. J. Monkhorst and J. D. Pack, *Physical review B* **13**, 5188 (1976).
  - [22] S. Dudarev, G. Botton, S. Savrasov, C. Humphreys, and A. Sutton, *Physical Review B* **57**, 1505 (1998).
  - [23] K.-H. Kim, H.-S. Kim, and M. J. Han, *J. Phys. Cond. Matter* **26**, 185501 (2014).
  - [24] A. Togo and I. Tanaka, *Scripta Materialia* **108**, 1 (2015).
  - [25] Y. Xie, H.-t. Yu, G.-x. Zhang, and H.-g. Fu, *Journal of Physics: Condensed Matter* **20**, 215215 (2008).
